# Supplementary material for: Exact Numerical Solution of Stochastic Master Equations for Conditional Spin Squeezing
Source: arXiv:2402.02495 source file (2024-02-04)
Supplement: Supplementary file 1 [file Supplemental_Material.pdf]

# Supplemental Material for Exact Numerical Solution of Stochastic Master Equations for Conditional Spin Squeezing

ZhiQing Zhang,<sup>1</sup> Yuan Zhang,<sup>1,2,\*</sup> HaiZhong Guo,<sup>1,2</sup> Chongxin Shan,<sup>1,2</sup> Gang Chen,<sup>1,2,†</sup>  
and Klaus Molmer<sup>3,‡</sup>

<sup>1</sup>*Henan Key Laboratory of Diamond Optoelectronic Materials and Devices, Key Laboratory of Material Physics Ministry of Education, School of Physics and Microelectronics, Zhengzhou University, Zhengzhou 450052, China*

<sup>2</sup>*Institute of Quantum Materials and Physics, Henan Academy of Sciences, Zhengzhou 450046, China*

<sup>3</sup>*Niels Bohr Institute, University of Copenhagen, 2100 Copenhagen, Denmark*

## CONTENTS

|                          |     |
|--------------------------|-----|
| S1. Parameters.cuh ..... | S1  |
| S2. Functions.cu .....   | S5  |
| S3. Functions.cuh .....  | S22 |
| S4. Dynamics.cu .....    | S24 |
| S5. Random.py .....      | S41 |

## S1. Parameters.cuh

```

1.      #if !defined(PARAMETERS)
2.      #define PARAMETERS
3.
4.      // !!!!!!!!!!!!!!!!!!!!!!!!!!!!!!!!!!!!!!!
5.      // we have to set the parameters as the micro variables
6.      // in this way, we do not need to pass the parameters to
7.      // the functions running on GPU
8.      //
9.      // the program for solving the master equations of spin
10.     // ensemble including individual and collective decay
11.     // and pumping as well as the coherent collective pumping
12.     // written by Yuan Zhang on 03. March 2017
13.     // contacted by yzhang
14.     // !!!!!!!!!!!!!!!!!!!!!!!!!!!!!!!!!!!!!!!
15.
16.
17.     #define PI 3.141592654
18.
19.     //!!!!!!!!!!!!!!!!!!!!!!
20.     // for the atoms
21.     //!!!!!!!!!!!!!!!!!!!!!!
22.     // transition frequency
23.     #define OMEGA_UD (0.)

```

```
24.
25. // freueqncy detunning
26. #define DELTA_UP (2.*PI*1.e9)
27. #define DELTA_DOWN (2.*PI*1.e9)
28.
29. // individual decay
30. // unit Hz
31. // real value
32. #define GAMMA (3.1e7)
33. //
34. //!!!!!!!!!!!!!!
35. // for the cavity mode
36. //!!!!!!!!!!!!!!
37. // damping rate of the cavity mode
38. // unit Hz
39. #define KAPPA (1.88e7)
40.
41. // atoms-cavity mode coupling
42. // unit Hz
43. #define GCOUP (0.94e7)
44.
45. // detection efficiencies
46. #define ETA (0.6)
47.
48. //!!!!!!!!!!!!!!
49. // incoming wave
50. //!!!!!!!!!!!!!!
```

```

51. // polarization along x direction
52. // amplitude
53. #define BETA_IN (1.2e2)
54.
55. // polarization angle
56. #define POLAR_ANG (0.0*PI)
57.
58. // initial values of angles to determine the
59. // initial states of the atoms
60. // pi/2 for spin coherent state
61. #define theta_init (0.5*PI)
62. // ground state
63. // #define theta_init (0.)
64. #define phi_init 0.
65.
66. // !!!!!!!!!!!!!!!!!!!!!!!!!!!!!!!!!!!!!!!
67. // 1. the dimension of reduced density matrix here
68. // 2. the configuration of threads in GPU
69. // !!!!!!!!!!!!!!!!!!!!!!!!!!!!!!!!!!!!!!!
70. // the demission of density matrix should be defined as a macro parameter but not a
    variable
71. // because we access this parameter in the functions run in GPU
72.
73. // number of spins
74. #define N_SPINS 100
75. // number of spin states to categorize density matrix elements
76. #define N_ELE ((N_SPINS+3)*(N_SPINS+2)*(N_SPINS+1)/6)

```

```

77.
78.     #define BASE (N_SPINS + 1)
79.     //!!!!!!!!!!!!!!!!!!!!!!!!!!!!!!!!!!!!!!
80.     // how we can calculate the index of the elements
81.     // we can connect each index with an number
82.
83.     //!!!!!!!!!!!!!!!!!!!!!!!!!!!!!!!!!!!!!!
84.
85.     // !!!!!!!!!!!!!!!!!!!!!!!!!!!!!!!!!!!!!!!
86.     // It is very essential to design how to use
87.     // the threads supported by specific NIVIDA graphe card.
88.     // For example, Telas M2050 has 448 physics corees
89.     // maximum number of threads per block: 1024
90.     // dimension of a block: 1024*1024*64
91.     // dimension of a grid: 63353*63353*63353
92.     // we use N_ELE threads, where the thread index specify
93.     // the collective states
94.     // It has N_ELE = 176851 collective states
95.     // threfore we have to utilize N_ELE/256= 690.82 blocks
96.     //
97.     // we utilize one linear block and linear threads configuration
98.     // it means that the global thread index can be calculated with
99.     // #define   id = blockIdx.x*blockDim.x + threadIdx.x
100.    // the collective state can be calculated with the block and thread index
101.    //
102.    // !!!!!!!!!!!!!!!!!!!!!!!!!!!!!!!!!!!!!!!
103.

```

```

104.    // the number of atoms should be smaller than "THREADS"
105.    // since we utilize the __syncthreads() to synchronize
106.    // the threads in the same block
107.
108.    #define THREADS 256
109.    #define BLOCKS N_ELE/256 +1
110.
111.    // The rest parameters
112.    // the number of matrix elements
113.    #define LENGTH_RHO N_ELE
114.    // time parameters
115.    // unit second
116.    // collective dephasing is about 10^5 Hz
117.    // therefore, our simulation time is about
118.    #define TIME_FINAL (1.e-5)
119.    // 2**16 = 65536 2**17 = 131072
120.    #define T_STEPS 65536
121.
122.    #define TIME_STEP (TIME_FINAL/T_STEPS)
123.    #define TIME_STORE 16*TIME_STEP
124.
125.    #endif

```

## S2. Functions.cu

```

1.    //all functions

```

```
2.      #include <math.h>
3.      #include <stdio.h>
4.      #include <assert.h>
5.      #include <cuda.h>
6.      #include <cuda_runtime.h>
7.      // parameters and functions
8.      #include "parameters.cuh"
9.      #include "functions.cuh"
10.
11.     using namespace std;
12.
13.
14.     __host__ __device__ int Fn(int n){
15.         int res;
16.         res = 1;
17.         for(int ind = 1; ind<=n; ind++){
18.             res = res*ind;
19.         }
20.         return res;
21.     }
22.
23.     // define 'combination' function
24.
25.     __host__ __device__ int CombMN(int up,int down) {
26.         int res,temp1,temp2;
27.         if ((up == 0) || (up == down)) res = 1;
28.         else {
```

```

29.     if ( up >= (down-up)) {
30.         temp1=Fn(down-up);
31.         temp2 = 1;
32.         for (int ind = up+1; ind<=down; ind++){
33.             temp2 = temp2*ind;
34.         }
35.         res = temp2/temp1;
36.     }
37.     if ( up < (down-up)) {
38.         temp1 = Fn(up);
39.         temp2 =1;
40.         for(int ind = down-up+1; ind <= down; ind++){
41.             temp2 = temp2*ind;
42.         }
43.         res = temp2/temp1;
44.     }
45. }
46. return res;
47. }
48.
49. __host__ __device__ int Fnk(int n, int k){
50.     return CombMN(k-1, n+k-1);
51. }
52.
53. __host__ __device__ int BallsBoxs(int n, int k) {
54.     int res;
55.     res=CombMN(k-1, n+k-1);

```

```

56.     return res;
57. }
58.
59. __host__ __device__ int Indics(int ndd, int ndu, int nud, int nuu){
60.     int ind = 1;
61.     if (nud-1 >= 0) {
62.         for(int i = 0; i<= nud-1; i++){
63.             ind += BallsBoxs(N_SPINS-ndd-ndu-i, 1);
64.         }
65.     }
66.     if (ndu-1 >= 0) {
67.         for(int i = 0; i<= ndu-1; i++){
68.             ind += BallsBoxs(N_SPINS-ndd-i, 2);
69.         }
70.     }
71.     if (ndd-1 >= 0) {
72.         for(int i = 0; i<= ndd-1; i++){
73.             ind += BallsBoxs(N_SPINS-i, 3);
74.         }
75.     }
76.     ind -= 1;
77.     return ind;
78. }
79.
80. __host__ __device__ int Knm(int n, int m) {
81.     int res = Fnk(n, m+1) - Fnk(n, m+2);
82.     return res;

```

```

83.     }

84.     //*****
85.     //   Initialization Functions
86.     //*****
87.     void initialization_double(double *in, int num){
88.         for (int i=0; i<num; i++){
89.             in[i] = 0.0;
90.         }
91.     }
92.
93.     void initialization_double2(double2 *in, int num){
94.         for (int i=0; i<num; i++){
95.             in[i].x = 0.0;
96.             in[i].y = 0.0;
97.         }
98.     }
99.
100.    __global__ void initialization(double2 *in1, double2 *in2){
101.        // calculate the index of matrix
102.        int ind = threadIdx.x + blockIdx.x*blockDim.x;
103.        if (ind < N_ELE) {
104.            in1[ind].x = 0.0;
105.            in1[ind].y = 0.0;
106.            in2[ind].x = 0.0;
107.            in2[ind].y = 0.0;

```

[illegible]

```

                                double2 xi_up, \double2 xi_down){
134.    // calculate the index of matrix
135.    int ind = threadIdx.x + blockIdx.x*blockDim.x;
136.
137.    // setup shared memory
138.    const int number_ds = 8*(N_SPINS+1);
139.    const int number_as = 3*(N_SPINS+1);
140.    __shared__ double data_shared[number_ds];
141.    __shared__ double angs_shared[number_as];
142.    __shared__ double ba_shared[N_SPINS+1];
143.
144.    // data to store calculated observables
145.    //  data[0] data[1]  data[2]  data[3]  data[4]  data[5]      data[6]    data[7]
146.    //   jx      jy      jz      uyx      uyy      uyz      current    pop
147.
148.
149.    // initialize the shared memory
150.    if(ind == 0){
151.        for (int nuu = 0; nuu <= N_SPINS; nuu ++){
152.            for (int nds = 0; nds <8; nds ++){
153.                data_shared[nuu*8+nds] = 0.;
154.            }
155.            for (int nas = 0; nas <3; nas ++){
156.                angs_shared[nuu*3+nas] = 0.;
157.            }
158.            ba_shared[nuu] = 0.;
159.        }

```

```

160.     }
161.     __syncthreads();
162.
163.
164.     if (ind <= N_SPINS){
165.         int index = Indics(N_SPINS - ind, 0, 0, ind);
166.
167.         // total population
168.         data_shared[ind*8+7] += com_dev[ind]*rho_dev[index].x;
169.
170.         // printf("%d %e\n", ind, com_dev[ind]);
171.
172.         // here because the binomial can be very huge, it can overflow the
173.         // randu of integer in c language, we can separate the calculations
174.         // to a loop
175.
176.         // jz
177.         data_shared[ind*8+2] += com_dev[ind]*ind*rho_dev[index].x;
178.
179.         if (ind >= 1){
180.             index = Indics(N_SPINS-ind, 1, 0, ind-1);
181.             // jx
182.             data_shared[ind*8+0] += 0.5*com_dev[ind]*ind*rho_dev[index].x;
183.             // jy
184.             data_shared[ind*8+1] -= 0.5*com_dev[ind]*ind*rho_dev[index].y;
185.         }
186.

```

```

187.     if ( ind <= N_SPINS -1){
188.         index = Indics(N_SPINS - ind-1, 0, 1, ind);
189.         // jx
190.         data_shared[ind*8+0] += 0.5*com_dev[ind]*(N_SPINS-ind)*rho_dev[index].x;
191.         // jy
192.         data_shared[ind*8+1] += 0.5*com_dev[ind]*(N_SPINS-ind)*rho_dev[index].y;
193.     }
194.
195.
196.     // for uncertainty of the jx,jy
197.     if (ind >1){
198.         index = Indics(N_SPINS-ind, 2, 0, ind-2);
199.         angs_shared[ind*3+0] += 0.25*com_dev[ind]*ind*(ind-1)*rho_dev[index].x;
200.         angs_shared[ind*3+1] -= 0.25*com_dev[ind]*ind*(ind-1)*rho_dev[index].x;
201.     }
202.
203.     index = Indics(N_SPINS-ind, 0, 0 , ind);
204.     angs_shared[ind*3+0] += 0.25*com_dev[ind]*N_SPINS*rho_dev[index].x;
205.     angs_shared[ind*3+1] += 0.25*com_dev[ind]*N_SPINS*rho_dev[index].x;
206.
207.     if (ind>0 && ind<N_SPINS){
208.         index = Indics(N_SPINS-ind-1, 1, 1, ind-1);
209.         angs_shared[ind*3+0] += 0.25*2*com_dev[ind]*ind*(N_SPINS-ind)*rho_dev[index].x;
210.         angs_shared[ind*3+1] += 0.25*2*com_dev[ind]*ind*(N_SPINS-ind)*rho_dev[index].x;
211.     }
212.
213.     if (ind <N_SPINS -1){

```

```

214.     index = Indics(N_SPINS-ind-2, 0, 2, ind);
215.     angs_shared[ind*3+0] +=
        0.25*com_dev[ind]*(N_SPINS-ind)*(N_SPINS-ind-1)*rho_dev[index].x;
216.     angs_shared[ind*3+1] -=
        0.25*com_dev[ind]*(N_SPINS-ind)*(N_SPINS-ind-1)*rho_dev[index].x;
217. }
218.
219. // for uncertainty of the jz
220. // combination up down up down
221. index = Indics(N_SPINS-ind, 0, 0, ind);
222. angs_shared[ind*3+2] +=
        0.25*com_dev[ind]*(2*ind-N_SPINS)*(2*ind-N_SPINS)*rho_dev[index].x;
223.
224. //
225. // measurement backactions
226. //
227. ba_shared[ind] += com_dev[ind]*(2.*xi_up.x*(N_SPINS-ind) +
        2.*xi_down.x*ind)*rho_dev[index].x;
228. }
229. __syncthreads();
230.
231. // calculate the sumed data
232. if (ind == 0){
233.
234.     for (int nds = 0; nds <8; nds++){
235.         data_dev[nds] = 0.;
236.         for (int nuu = 0; nuu <= N_SPINS; nuu++){

```

```

237.         data_dev[nds] += data_shared[nuu*8+nds];
238.     }
239. }

240.     data_dev[2] -= 0.5*N_SPINS;
241.
242.     double angs[3];
243.     for (int nas = 0; nas <3; nas++){
244.         angs[nas] = 0.;
245.         for (int nuu = 0; nuu <= N_SPINS; nuu++){
246.             angs[nas] += angs_shared[nuu*3+nas];
247.         }
248.     }
249.
250.     // uncertainty of angular momentum
251.     data_dev[3] = sqrtf(angs[0]-data_dev[0]*data_dev[0]);
252.     data_dev[4] = sqrtf(angs[1]-data_dev[1]*data_dev[1]);
253.     data_dev[5] = sqrtf(angs[2]-data_dev[2]*data_dev[2]);
254.
255.     *ba_dev = 0.;
256.     for (int nuu = 0; nuu <= N_SPINS;nuu++){
257.         *ba_dev += ba_shared[nuu];
258.     }
259.
260.     // calculate the homodyne detection signal
261.     data_dev[6] = *ba_dev + rn_dev/TIME_STEP;

```

```

262.     }
263.     __syncthreads();
264.     }
265.
266.     //*****
267.     //    dynamics and measure backactions
268.     //*****
269.     // define the main function running in GPU side
270.     __global__ void dynamics_backactions(double2 *rho_dev, double2 *drho_sdt_dev, \
271.                                         double2 *rho_ba_dev,  int *mapmap_dev,\
272.                                         double *ba_dev,double rn_dev, \
273.                                         double chi_up,    double chi_down, \
274.                                         double2 xi_up, double2 xi_down, double time){
275.         // calculate the index of matrix
276.         int ind = threadIdx.x + blockIdx.x*blockDim.x;
277.
278.         if (ind < N_ELE) {
279.
280.             // here x indicates the base
281.             //    nuu    nud    ndu    ndd
282.             //    n0     n1     n2     n3
283.
284.             // collective quantum number
285.             int nab[4];
286.
287.             // calculate the coefficients of the expansion
288.             int num = mapmap_dev[ind];

```

```

289.
290.     // here we can determine the four numbers related to
291.     // the index
292.     for (int i=0; i<=3; i++){
293.         nab[i] = num%BASE;
294.         num = num/BASE;
295.     }
296.     int nuu = nab[0]; int nud = nab[1];
297.     int ndu = nab[2]; int ndd = nab[3];
298.
299.     // here printf("ind = %d, vector %d %d %d %d \n",ind,ndd,ndu,nud,nuu);
300.
301.     // the quesiton is how to effectively determine the index
302.     // if we know the collective numbers
303.     //
304.     // the easiest way is to
305.     // calculate the integer from the collective numbers
306.     // by searching the array, we can identiy the index
307.     //
308.     // based on the arrandument of the elements, we may
309.     // calculate the index based on the present index
310.
311.     double temp;
312.     double2 temp2;
313.     int index;
314.
315.     //*****

```

```

316. // dynamics
317. //*****
318.
319. drho_sdt_dev[ind].x = 0.; drho_sdt_dev[ind].y = 0.;
320.
321. //////////////////////////////////////
322. // transition energy and stark energy shift
323. //////////////////////////////////////
324.
325. /* in the rotation framework
326. temp = (OMEGA_UD + 2.*DELTA_UP*chi_up - 2.*DELTA_DOWN*chi_down)*(ndu-nud);
327. drho_sdt_dev[ind].x += temp*rho_dev[ind].y;
328. drho_sdt_dev[ind].y -= temp*rho_dev[ind].x;
329. */
330.
331. //////////////////////////////////////
332. // dephasing rate of individual atoms
333. //////////////////////////////////////
334.
335. temp = (1. / 3.) * GAMMA * (chi_up + chi_down) * (ndu + nud);
336. drho_sdt_dev[ind].x -= temp * rho_dev[ind].x;
337. drho_sdt_dev[ind].y -= temp * rho_dev[ind].y;
338.
339. //////////////////////////////////////
340. // pumping rate of individual atoms
341. //////////////////////////////////////
342. temp = (1. / 6.) * GAMMA * chi_up * (ndu + nud);

```

```

343.     drho_sdt_dev[ind].x -= temp * rho_dev[ind].x;
344.     drho_sdt_dev[ind].y -= temp * rho_dev[ind].y;
345.
346.     temp = (1. / 3.) * GAMMA * chi_up;
347.     drho_sdt_dev[ind].x -= temp * ndd * rho_dev[ind].x;
348.     drho_sdt_dev[ind].y -= temp * ndd * rho_dev[ind].y;
349.
350.     if (nuu - 1 >= 0)
351.     {
352.         //index = Indics(ndd+1,ndu,nud,nuu-1);n
353.         index = ind - Knm(N_SPINS - ndd, 1) - Knm(N_SPINS - ndd - ndu, 0)\
354.             + Fnk(N_SPINS - ndd - ndu - nud, 1);
355.         //printf("index %d is equal to %d \n",index,index_com);
356.
357.         drho_sdt_dev[ind].x += temp * nuu * rho_dev[index].x;
358.         drho_sdt_dev[ind].y += temp * nuu * rho_dev[index].y;
359.     }
360.
361.
362.     //////////////////////////////////////
363.     // decay rate of individual atoms
364.     //////////////////////////////////////
365.     temp = (1. / 6.) * GAMMA * chi_down * (ndu + nud);
366.     drho_sdt_dev[ind].x -= temp * rho_dev[ind].x;
367.     drho_sdt_dev[ind].y -= temp * rho_dev[ind].y;
368.
369.     temp = (1. / 3.) * GAMMA * chi_down;

```

```

370.     drho_sdt_dev[ind].x -= temp * nuu * rho_dev[ind].x;
371.     drho_sdt_dev[ind].y -= temp * nuu * rho_dev[ind].y;
372.
373.     if (nnd - 1 >= 0)
374.     {
375.         index = Indics(nnd - 1, ndu, nud, nuu + 1);
376.         //index = ind + Knm(N_SPINS-nnd+1,1)\
377.             +Knm(N_SPINS-nnd-ndu+1,0)-Fnk(N_SPINS-nnd-ndu-nud+1,1);
378.         //printf("index %d is equal to %d \n",index,index_com);
379.
380.         drho_sdt_dev[ind].x += temp * nnd * rho_dev[index].x;
381.         drho_sdt_dev[ind].y += temp * nnd * rho_dev[index].y;
382.     }
383.
384.
385.     ////////////////////////////////////////////
386.     // collective dephasing rate
387.     ////////////////////////////////////////////
388.     temp = (2.*GCOUP*GCOUP/KAPPA)*(chi_up + chi_down)*(ndu - nud)*(ndu - nud);
389.     drho_sdt_dev[ind].x -= temp*rho_dev[ind].x;
390.     drho_sdt_dev[ind].y -= temp*rho_dev[ind].y;
391.
392.
393.     //*****
394.     // measurement backactions
395.     //*****
396.     rho_ba_dev[ind].x = 0.; rho_ba_dev[ind].y = 0.;

```

```

397.
398.
399.     rho_ba_dev[ind].x -= rn_dev>(*ba_dev)*rho_dev[ind].x;
400.     rho_ba_dev[ind].y -= rn_dev>(*ba_dev)*rho_dev[ind].y;
401.
402.     temp2.x = xi_up.x*(ndd+nud) + xi_up.x*(ndd + ndu) \
403.             + xi_down.x*(nuu+ndu) + xi_down.x*(nud + nuu);
404.
405.     temp2.y = xi_up.y*(ndd+nud) - xi_up.y*(ndd + ndu) \
406.             + xi_down.y*(nuu+ndu) - xi_down.y*(nud + nuu);
407.
408.     rho_ba_dev[ind].x += rn_dev*(temp2.x*rho_dev[ind].x - temp2.y*rho_dev[ind].y);
409.     rho_ba_dev[ind].y += rn_dev*(temp2.x*rho_dev[ind].y + temp2.y*rho_dev[ind].x);
410.
411. }
412.
413. }
414.
415. //*****
416. // calculate the new density matrix
417. //*****
418. __global__ void update_rho(double2 *rho_dev,double2 *rho_old_dev,\
419.                            double2 *drho_sdt_dev,double2 *rho_ba_dev){
420. // calculate the index of matrix
421. int ind = threadIdx.x + blockIdx.x*blockDim.x;
422. if (ind < N_ELE) {
423.     rho_dev[ind].x = rho_old_dev[ind].x + TIME_STEP*drho_sdt_dev[ind].x\

```

```

424.          + rho_ba_dev[ind].x;
425.    rho_dev[ind].y = rho_old_dev[ind].y + TIME_STEP*drho_sdt_dev[ind].y\
426.          + rho_ba_dev[ind].y;
427.    }
428.    }

```

### S3. Functions.cuh

```

1.    //all functions
2.    #if !defined(FUNCTIONS_H)
3.    #define FUNCTIONS_H
4.
5.    #include <cuda.h>
6.    #include <stdio.h>
7.    #include "parameters.cuh"
8.    #include "functions.cuh"
9.
10.   using namespace std;
11.
12.   __host__ __device__ int Fn(int n);
13.
14.   // define 'combination' function
15.   __host__ __device__ int CombMN(int up, int down);
16.
17.   __host__ __device__ int BallsBoxs(int n, int k);
18.

```

```

19.  __host__ __device__ int Indics(int ndd, int ndu, int nud, int nuu);
20.
21.  __host__ __device__ int Knm(int n, int m);
22.
23.  __host__ __device__ int Fnk(int n, int k);
24.
25.  __global__ void initialization(double2 *in1, double2 *in2);
26.
27.
28.  //*****
29.  // copy the reduced density matrix
30.  //*****
31.
32.  __global__ void copy_rho(double2 *rho1, double2 *rho2);
33.
34.
35.  //*****
36.  // calculate observables
37.  //*****

38.  __global__ void observables(double2 *rho_dev, double *ba_dev, double rn_dev, \
39.                             double *data_dev, double *com_dev, double2 xi_up, \
40.                             double2 xi_down);
41.
42.  //*****
43.  //  dynamics and backactions

```

```

44. //*****
45. // define the main function running in GPU side
46.
47. __global__ void dynamics_backactions(double2 *rho_dev, double2 *drho_sdt_dev, \
48.                                     double2 *rho_ba_dev, int *mapmap, \
49.                                     double *ba_dev, double rn_dev, \
50.                                     double chi_up, double chi_down, \
51.                                     double2 xi_up, double2 xi_down, double time);
52.
53. //*****
54. //   update rho
55. //*****
56.
57. __global__ void update_rho(double2 *rho_dev, double2 *rho_old_dev, \
58.                            double2 *drho_sdt_dev, double2 *rho_ba_dev);
59.
60. #endif

```

#### S4. Dynamics.cu

```

1. /*
2.   Code to propagate the reduced density matrix
3.   with Rundu-Kutta method in CUDA language
4.
5.   written by Yuan Zhang, date 03.03.2017.
6.   email: yzhuaudipc@163.com

```

7. for the explanation, see related pdf file.  
8.  
9. the program for solving the master equations of spin  
10. ensemble including individual and collective decay  
11. and pumping as well as the coherent collective pumping  
12. written by Yuan Zhang on 03. March 2017  
13.  
14. all the parameters are summarized in the file "parameters.cu"  
15. all the functions are summarized in the file "functions.cu"  
16. \*/  
17.  
18.  
19. #include <math.h>  
20. #include <io.h>  
21. #include <process.h>  
22. #include <stdlib.h>  
23. #include <stdio.h>  
24. #include <cuda.h>  
25. #include <ctime>  
26. #include <curand\_kernel.h>  
27. #include <curand.h>  
28. #include "parameters.cuh"  
29. #include "functions.cuh"  
30.  
31.  
32. // check program  
33.

```

34.
35.     #define gpuErrchk(ans) { gpuAssert((ans), __FILE__, __LINE__); }
36.     inline void gpuAssert(cudaError_t code, const char *file, int line, bool abort=true)
37.     {
38.         if (code != cudaSuccess)
39.         {
40.             fprintf(stderr,"GPUassert: %s %s %d\n", cudaGetErrorString(code), file, line);
41.             if (abort) exit(code);
42.         }
43.     }

44.     // gpuErrchk( cudaPeekAtLastError() );
45.     // gpuErrchk( cudaDeviceSynchronize() );
46.
47.
48.     // *****
49.     // main function
50.     // *****
51.
52.     int main(void){
53.
54.         // calculate the time nuuded for the program
55.         clock_t ct0,ct1;
56.         ct0 = clock();
57.
58.

```

```

59.      // open the files to store the data
60.      FILE *of_time, *of_ang_mom, *of_squeezing, *of_cur;
61.      // time of simulation
62.      of_time = fopen("DATA/time.dat","w");
63.      // angular momenta
64.      of_ang_mom= fopen("DATA/ang_mom.dat", "w");
65.      // spin squeezing parameters
66.      of_squeezing = fopen("DATA/squeezing.dat", "w");
67.      // homodyne detection current
68.      of_cur = fopen("DATA/cur.dat", "w");
69.
70.
71.      // combination numbers
72.      double com[N_SPINS+1];
73.      // biol down the binomial
74.      int down = N_SPINS;
75.      for (int up = 0; up<=N_SPINS; up++){
76.          if ((up == 0) || (up == down)) com[up] = 1.;
77.          else {
78.              if ( up >= (down-up)) {
79.                  double temp1=1., temp2=1.;
80.                  for (int ind_acc = 1; ind_acc <= down-up; ind_acc++){
81.                      temp1 = temp1*ind_acc;
82.                      temp2 = temp2*(up+ind_acc);
83.                  }
84.                  com[up]  = temp2/temp1;
85.              }

```

```

86.         if ( up < (down-up)) {
87.             double temp1=1., temp2=1.;
88.             for (int ind_acc = 1; ind_acc <= up; ind_acc++){
89.                 temp1 = temp1*ind_acc;
90.                 temp2 = temp2*(down-up+ind_acc);
91.             }
92.             com[up] = temp2/temp1;
93.         }
94.     }
95. }
96. // *****
97. // copy the com from CPU side to GPU side
98. // *****
99. int size_com = (N_SPINS+1)*sizeof(double);
100. double *com_dev;
101. cudaMalloc((void**)&com_dev, size_com);
102. cudaMemcpy(com_dev,com, size_com, cudaMemcpyHostToDevice);
103.
104.
105. // compute the map of the numbers
106. int mapmap[N_ELE];
107. int base[4];
108. base[0] = 1;
109. for (int i=1; i<=3; i++){
110.     base[i] = base[i-1]*BASE;
111. }
112.

```

```

113.
114.     int ind = 0;
115.     for (int ndd = 0; ndd <= N_SPINS; ndd++){
116.         for (int ndu = 0; ndu <= N_SPINS-ndd; ndu++){
117.             for (int nud = 0; nud <= N_SPINS-ndd-ndu; nud++){
118.                 int nuu = N_SPINS-ndd-ndu-nud;
119.                 // code the three numbers to one number
120.                 mapmap[ind] = ndd*base[3] + ndu*base[2] \
121.                 + nud*base[1] + nuu*base[0];
122.                 //      printf("ind = %d, vector %d %d %d %d \n", ind, nuu, nud, ndu, ndd);
123.                 ind = ind + 1;
124.             }
125.         }
126.     }
127.
128.
129.
130.     // *****
131.     // copy the mapmap from CPU side to GPU side
132.     // *****
133.
134.     int *mapmap_dev;
135.     int size_map = N_ELE*sizeof(int);
136.     cudaMalloc((void**)&mapmap_dev,size_map);
137.     cudaMemcpy(mapmap_dev, mapmap, size_map, cudaMemcpyHostToDevice);
138.
139.

```

```

140. // *****
141. // initialize the reduced density matrix in CPU side
142. // *****
143. // total number of reduced density matrix elements
144.
145. int size_rho = N_ELE*sizeof(double2);
146.
147. // assign the memory for the reduced density matrix in CPU and GPU side
148. double2 *rho = (double2 *)malloc(size_rho);
149. double2 *rho_old = (double2 *)malloc(size_rho);
150.
151.
152. for (int ind=0;ind < N_ELE;ind++){
153.     rho[ind].x = 0.;
154.     rho[ind].y = 0.;
155.     rho_old[ind].x=0.;
156.     rho_old[ind].y=0.;
157. }
158.
159.
160. // initialization of the reduced density matrix
161. // determine the initial states of the atoms
162. // with two angles, theta, phi
163. double2 c1,c2;
164. c1.x = cos(0.5*theta_init); c1.y = 0.;
165. c2.x = sin(0.5*theta_init)*cos(phi_init); c2.y = sin(0.5*theta_init)*sin(phi_init);
166. double2 c1c1s, c2c2s, c1c2s, c2c1s;

```

```

167.     c1c1s.x = c1.x*c1.x + c1.y*c1.y; c1c1s.y = 0.;
168.     c2c2s.x = c2.x*c2.x + c2.y*c2.y; c2c2s.y = 0.;
169.     c1c2s.x = c1.x*c2.x + c1.y*c2.y; c1c2s.y = - c1.x*c2.y + c1.y*c2.x;
170.     c2c1s.x = c2.x*c1.x + c2.y*c1.y; c2c1s.y = - c2.x*c1.y + c2.y*c1.x;
171.
172.
173.     double2 temp, temp1;
174.     for (int ndd = 0; ndd <= N_SPINS; ndd++){
175.         for (int ndu = 0; ndu <= N_SPINS-ndd; ndu++){
176.             for (int nud = 0; nud <= N_SPINS-ndd-ndu; nud++){
177.                 int nuu = N_SPINS-ndd-ndu-nud;
178.
179.                 temp.x = 1.; temp.y = 0.;
180.                 if ( nuu>0) {
181.                     for (int nj = 1; nj <= nuu; nj++){
182.                         temp1.x = temp.x; temp1.y = temp.y;
183.                         temp.x = temp1.x*c2c2s.x - temp1.y*c2c2s.y;
184.                         temp.y = temp1.x*c2c2s.y + temp1.y*c2c2s.x;
185.                     }
186.                 }
187.                 if ( nud>0) {
188.                     for (int nj = 1; nj <= nud; nj++){
189.                         temp1.x = temp.x; temp1.y = temp.y;
190.                         temp.x = temp1.x*c2c1s.x - temp1.y*c2c1s.y;
191.                         temp.y = temp1.x*c2c1s.y + temp1.y*c2c1s.x;
192.                     }
193.                 }

```

```

194.         if ( ndu>0) {
195.             for (int nj = 1; nj <= ndu; nj++){
196.                 temp1.x = temp.x; temp1.y = temp.y;
197.                 temp.x = temp1.x*c1c2s.x - temp1.y*c1c2s.y;
198.                 temp.y = temp1.x*c1c2s.y + temp1.y*c1c2s.x;
199.             }
200.         }
201.         if ( ndd>0) {
202.             for (int nj = 1; nj <= ndd; nj++){
203.                 temp1.x = temp.x; temp1.y = temp.y;
204.                 temp.x = temp1.x*c1c1s.x - temp1.y*c1c1s.y;
205.                 temp.y = temp1.x*c1c1s.y + temp1.y*c1c1s.x;
206.             }
207.         }
208.
209.         int ind = Indics(ndd,ndu,nud,nuu);
210.         rho[ind].x = temp.x;
211.         rho[ind].y = temp.y;
212.     }
213. }
214. }
215.
216.
217. //*****
218. // calcualte other combined parameters
219. //*****
220. double beta_up, beta_down;

```

```

221.    beta_up = cos(POLAR_ANG)*BETA_IN;
222.    beta_down = sin(POLAR_ANG)*BETA_IN;
223.
224.
225.    double chi_up = beta_up*beta_up*GCOUP*GCOUP\
226.                  /(DELTA_UP*DELTA_UP+0.25*GAMMA*GAMMA);
227.
228.    double chi_down = beta_down*beta_down*GCOUP*GCOUP\
229.                  /(DELTA_DOWN*DELTA_DOWN+0.25*GAMMA*GAMMA);
230.
231.    double2 xi_up, xi_down;
232.
233.    temp.x = (beta_up/BETA_IN)*sqrtf(ETA*KAPPA)*(2*GCOUP/KAPPA)\
234.            *(beta_up*GCOUP/(DELTA_UP*DELTA_UP+0.25*GAMMA*GAMMA));
235.    xi_up.x = temp.x*DELTA_UP;
236.    xi_up.y = temp.x*(0.5*GAMMA);
237.
238.    temp.x = (beta_down/BETA_IN)*sqrtf(ETA*KAPPA)*(2*GCOUP/KAPPA)\
239.            *(beta_down*GCOUP/(DELTA_DOWN*DELTA_DOWN+0.25*GAMMA*GAMMA));
240.    xi_down.x = temp.x*DELTA_DOWN;
241.    xi_down.y = temp.x*(0.5*GAMMA);
242.
243.
244.    //*****
245.    // list the parameters
246.    //*****

```

```

247.     printf("Simulation Parameters \n");
248.     printf("chi_up %e chi_down %e \n",chi_up,chi_down);
249.     // individual decay and pumping
250.     printf("individual decay and pumping %e   %e
\n",chi_up*GAMMA,chi_down*GAMMA);
251.     // collective dephasing
252.     printf("collective dephasing %e   %e\n",\
253.         chi_up*4*GCOUP*GCOUP/KAPPA, chi_down*4*GCOUP*GCOUP/KAPPA);
254.
255.     printf("xi_up: %e %e;xi_down: %e %e \n", xi_up.x, xi_up.y, xi_down.x, xi_down.y);

256.
257.     // simulation time
258.     printf("simulation time %e \n",TIME_FINAL);
259.
260.     printf("\n Press Any Key to Continue\n");
261.     getchar();

262.     // time parameters
263.     double time_sim = 0.;
264.
265.     // *****
266.     // copy the matrices from CPU side to GPU side
267.     // *****
268.     double2 *rho_dev,*rho_old_dev;
269.     cudaMalloc((void**)&rho_dev, size_rho);
270.     cudaMalloc((void**)&rho_old_dev, size_rho);

```

```

271.
272.     cudaMemcpy(rho_dev, rho, size_rho, cudaMemcpyHostToDevice);
273.     cudaMemcpy(rho_old_dev, rho_old, size_rho, cudaMemcpyHostToDevice);
274.
275.
276.     // *****
277.     // dynamics and measurement backactions
278.     // *****
279.
280.     double2 *drho_sdt_dev, *rho_ba_dev;
281.     // assign the memory for the variables used in rk4 method
282.     cudaMalloc((void**)&drho_sdt_dev, size_rho);
283.     cudaMalloc((void**)&rho_ba_dev, size_rho);
284.
285.     // backaction, random number
286.     double *ba_dev, *wt_dev;
287.     cudaMalloc((void**)&ba_dev, sizeof(double));
288.     cudaMalloc((void**)&wt_dev, sizeof(double));
289.
290.     // data to store calculated observables
291.     //  data[0] data[1]  data[2]  data[3]  data[4]  data[5]      data[6]    data[7]
292.     //   jx      jy      jz      uyx      uyy      uyz      current    pop
293.
294.     int size_data = 8*sizeof(double);
295.     double *data = (double *)malloc(size_data);
296.     double *data_dev;
297.     cudaMalloc((void**)&data_dev, size_data);

```

```

298.
299.     double *angs_dev;
300.     cudaMalloc((void**)&angs_dev, 3*sizeof(double));
301.
302.     // total number of random numbers
303.     int size_rn = T_STEPS*sizeof(double);
304.     double *rn = (double *)malloc(size_rn);
305.
306.     FILE *of_rn;
307.     of_rn = fopen("random_number.dat","r");
308.     for (int ind=0;ind < T_STEPS;ind++){
309.         fscanf(of_rn,"%lf \n", &rn[ind]);
310.         // printf("%e \n", rn[ind]);
311.     }
312.     fclose(of_rn);
313.
314.     // *****
315.     // simulations starts
316.     // *****
317.
318.     // update the old reduced density matrix
319.     for (int t = 1; t < T_STEPS; t++){
320.
321.         // copy rho to rho_old
322.         copy_rho<<<BLOCKS,THREADS>>>(rho_old_dev,rho_dev);
323.         cudaThreadSynchronize();
324.

```

```

325.         initialization<<<BLOCKS,THREADS>>>(drho_sdt_dev,rho_ba_dev);
326.         cudaThreadSynchronize();
327.
328.         // calculate observables
329.         observables<<<1,N_SPINS+1>>>(rho_dev,ba_dev,rn[t],data_dev,com_dev, \
330.                                     xi_up,xi_down);
331.         cudaThreadSynchronize();
332.
333.         // calculate dynamics and backactions
334.         dynamics_backactions<<<BLOCKS,THREADS>>>(rho_dev, drho_sdt_dev, \
335.                                                    rho_ba_dev, mapmap_dev,\
336.                                                    ba_dev, rn[t], chi_up, chi_down, \
337.                                                    xi_up, xi_down, time_sim);
338.         cudaThreadSynchronize();
339.
340.         // update rho
341.         update_rho<<<BLOCKS,THREADS>>>(rho_dev, rho_old_dev, drho_sdt_dev, \
342.                                         rho_ba_dev);
343.         cudaThreadSynchronize();
344.
345.
346.         // *****
347.         // copy the calculate observables back to CPU side
348.         // *****
349.
350.         if ( t%TIME_STORE == 0) {
351.

```

```

352.    // data[0] data[1] data[2] data[3] data[4] data[5] data[6] data[7]
353.    // jx      jy      jz      uyx      uyy      uyz      current      pop
354.    cudaMemcpy(data,data_dev,size_data,cudaMemcpyDeviceToHost);
355.
356.    // *****
357.    // store the physical observables
358.    // *****
359.    // time
360.    fprintf(of_time,"%e %e\n",(double)time_sim,data[7]);
361.
362.    // angular momenta
363.    fprintf(of_ang_mom,"%e %e %e %e %e %e \n", data[0], data[1], data[2], data[3],
364.    data[4], data[5]);
365.
366.    // current
367.    fprintf(of_cur, "%e \n", data[6]);
368.    // total population
369.    printf("%e\t %e\n", 100*(time_sim/TIME_FINAL), data[7]);
370.
371.    // calculate the squeezing parameters
372.    double squeezing[3];
373.    squeezing[0] = N_SPINS*data[3]*data[3]/(data[1]*data[1] + data[2]*data[2]);
374.    squeezing[1] = N_SPINS*data[4]*data[4]/(data[0]*data[0] + data[2]*data[2]);
375.    squeezing[2] = N_SPINS*data[5]*data[5]/(data[0]*data[0] + data[1]*data[1]);
376.
377.    // squeezing parameters
378.    fprintf(of_squeezing,"%e %e %e \n", squeezing[0], squeezing[1], squeezing[2]);

```

```

379.     }
380.         time_sim += TIME_STEP;
381.     }
382.
383.     // *****
384.     // store steady-state RDM for calculation of emission
385.     // *****
386.     cudaMemcpy(rho,rho_dev, size_rho, cudaMemcpyDeviceToHost);
387.
388.     FILE *of_rdm;
389.     of_rdm = fopen("DATA/rdm.dat","w");
390.     for (int ind=0; ind < N_ELE; ind++){
391.         fprintf(of_rdm, "%e \t %e \n", rho[ind].x, rho[ind].y);
392.     }
393.     fclose(of_rdm);
394.
395.     // free the rhos
396.     free(rho);
397.     free(rho_old);
398.
399.     cudaFree(rho_dev);
400.     cudaFree(rho_old_dev);
401.     cudaFree(drho_sdt_dev);
402.     cudaFree(rho_ba_dev);
403.
404.     //cudaFree(states_dev);
405.     cudaFree(ba_dev);

```

```
406.     cudaFree(wt_dev);
407.
408.     // free data
409.     free(data);
410.     cudaFree(data_dev);
411.
412.     // free com and mapmap
413.     cudaFree(com_dev);
414.     cudaFree(mapmap_dev);
415.
416.     // close the opened files
417.     fclose(of_time);
418.     fclose(of_ang_mom);
419.     fclose(of_squeezing);
420.     fclose(of_cur);
421.
422.     ct1=clock();
423.     fprintf(stderr, "Program takes about %.2f s\n",
424.             (double)(ct1-ct0)/(double)CLOCKS_PER_SEC);
425.
426.     printf("I am here! \n");
427.
428.     return 0;
429. }
```

**S5. Random.py**

```
1.      import numpy as np
2.
3.      TIME_FINAL = 1.e-5
4.      T_STEPS = 65536
5.      TIME_STEP = TIME_FINAL/T_STEPS
6.      mu,sigma = 0, np.sqrt(TIME_STEP)
7.      rn = np.random.normal(mu,sigma,T_STEPS)
8.      np.savetxt("random_number.dat",rn)
```
